# Supplementary material for: Two Burning Questions on COVID-19: Did shutting down the economy help? Can we (partially) reopen the economy without risking the second wave?
Source: arXiv:2005.00072 source file (2020-05-10)
Supplement: Supplementary file 1 [file si_covid.tex]

% SI FOR COVID        
\section{A Case Study in the Context of COVID-19}
In this section, we describe an application of Synthetic Interventions in the context of COVID-19. Before we present our empirical results, however, we first describe a high-level, abstract overview of the Synthetic Interventions algorithm -- specifically, the necessary input requirements and corresponding output. Then, through a case study that investigates the impact of mobility-restricting interventions on a country's death count, we formalize the overview by detailing the ins and outs of applying the Synthetic Interventions algorithm via an example. For the interested reader, we relegate the mathematical details of the algorithm to Section \ref{sec:alg}. 

% overview
\subsection{Overview of Synthetic Interventions Method} 

% input
\paragraph{Input.}
We consider the setting where there are $N$ units and $D$ possible interventions that can be applied towards each unit. For each unit, we have access to a time series of $T$ observations\footnote{The observations do not have to be indexed by time; rather, we only require $T$ measurements for each of the $N$ units.} according to some outcome variable of interest. Typically, the observed time series associated with each unit corresponds to only one of the $D$ interventions. 

% output
\paragraph{Output.} 
The output of the Synthetic Interventions algorithm is simply an augmentation of the observed data under all possible interventional scenarios. That is, the Synthetic Interventions algorithm predicts the counterfactual trajectory of the outcome variable under all $D$ interventions for every unit. If the counterfactual predictions are accurate and reliable, then a practitioner now has insights as to how each intervention affects every unit and the trade-offs between interventions, which can be unit-specific. 

% algorithm 
\paragraph{Algorithmic Intuition.}
For any {\em target} unit of interest, the Synthetic Interventions algorithm predicts the corresponding counterfactual trajectory of outcome variables under all unobserved interventions by leveraging observations from other {\em donor} units, which have enacted these interventions. That is, in order to predict the counterfactual observations for our target unit under any unobserved intervention, we first construct a ``synthetic'' version of our target unit as a weighted combination of donor units that received this intervention. Then, we use the ``synthetic'' target unit, along with the observations of our donor units under our intervention of interest, to create its counterfactual trajectory in this parallel setting. 

% fine print
\paragraph{Fine Print.} 
As previously mentioned, the input time series associated with each unit is typically associated with only one of the $D$ interventions. Hence, the foremost item that needs to be addressed is having a well-defined notion of an intervention.

Further, it is critical to specify an interventional point, which we will denote as $T_0 < T$; this event splits the time horizon of $T$ observations into a pre- and post-intervention period. Importantly, during the pre-intervention period (time points $t \le T_0$), which corresponds to all time points prior to the intervention, all units are assumed to be operating under a common setting (this could be the absence of any intervention or a shared intervention); this allows the algorithm to fairly (and accurately) build synthetic versions of each target unit from its donor units. During the post-intervention (time points $t > T_0$) period, however, each unit can now receive one of the $D$ interventions. The aim of Synthetic Interventions is to then predict how each unit would have behaved under all of the other unobserved interventions. 

From a data science perspective, there are several ``hyper-parameters'' for the Synthetic Interventions algorithm. First, is an appropriate definition of an intervention, and the corresponding intervention point to create a pre- and post-intervention period, which are used to build a model (synthetic versions of units) and make counterfactual predictions, respectively. Additionally, there is flexibility in defining the donor pool for every target unit, i.e., the candidate units used to build synthetic versions of the target units. In what follows, we will provide examples on how to address these issues.

% COVID-19
\subsection{COVID-19 Case Study} 
We are now ready to apply the Synthetic Interventions algorithm. In particular, we will use the Synthetic Interventions algorithm to predict how different interventions affect the number of COVID-19 related deaths within a country, i.e., we use  daily death count reports as our outcome variable of interest to measure a country's physical health. 

\paragraph{Defining Mobility Levels as Interventions.} 

Since many countries have implemented numerous policies simultaneously to combat the spread of COVID-19, it is difficult to analyze any particular policy (say stay-at-home) in isolation. However, if we consider the causal chain of events, then we observe that policies often affect how individuals move and interact, which then affects the spread and, ultimately, deaths associated with COVID-19. 
In light of this observation, we 
adopt mobility as our notion of intervention, and investigate how a country's mobility level translates to the number of potential COVID-19 related deaths\footnote{
To resolve any potential ambiguities, we will henceforth refer to interventions as the level of mobility within a country, and policies with orders such as the closing of schools or theomt enforcing of individuals to stay at home.
}.

To that end, we use Google's mobility data \cite{google_mobility} to measure a country's mobility and construct four different levels of mobility corresponding to four distinct interventions, which we define as follows:

\begin{itemize}
    \item[(a)] No mobility-restricting intervention: reduction in mobility is below $5\%$ compared to national baseline from January 2020.
    
    \item[(b)] Moderate mobility-restricting intervention: reduction in mobility is between $5\% - 30\%$ compared to national baseline from January 2020.
    
    \item[(c)] Strict mobility-restricting intervention: reduction in mobility is between $30\% - 50\%$ compared to national baseline from January 2020.
    
    \item[(d)] Very Strict mobility-restricting intervention: reduction in mobility is greater than $50\%$ compared to national baseline from January 2020.
\end{itemize}

\paragraph{Defining the Pre- and Post-Intervention Periods.} Recall that $T_0$ denotes our intervention point, which splits our time series of $T$ observations per country into a pre- and post-intervention period. However, rather than aligning all countries by the same chronological time points (i.e., actual dates), we will mark $T_0$ as the point at which $80$ deaths have occurred within the country. As a result, the chronological date at which the morbid event of $80$ deaths occurring may vary from country to country, but the definition of $T_0$ will remain consistent, i.e., the pre-intervention period for a country will correspond to the $T_0$ days prior to the $80$-th death within the country, and the post-intervention period will correspond to the $T-T_0$ days after.

\paragraph{Defining the Donor Pool.} 
Based on our definition of interventions, we will partition our $N$ countries into one of four buckets depending on the countries' levels of mobility during the post-intervention period (the time horizon after the $80$-th death). 
Thus, the aim of Synthetic Interventions is to predict the counterfactual death counts for each country under the other unobserved levels of mobility.

\paragraph{Counterfactual Predictions \& Evaluations.} 
To evaluate the efficacy of the Synthetic Interventions algorithm, we will measure its ability to recreate the observed death count trajectories for each country during the post-intervention period. 

\paragraph{Key Takeaways.} 

% As we can see in Figures...
% Since our predictions closely follow the actual death trajectories, our counterfactual predictions under the unobserved scenarios give insight as to how the death counts would have evolved had the countries operated under different levels of mobility. 

% % Statistical Details
% \subsection{Statistical Details and Further Examples}

% % abstract algorithm
% \subsubsection{Meta-Algorithm} 

% % hypothesis test
% \subsubsection{When {\em not} to use Synthetic Interventions}

% \begin{itemize}
%     \item Abstract algorithm
%     \item Hypothesis tests
%     \item Other examples - Economic stuff that Cindy did
%     \item Github repo forward pointer - work in progress 
% \end{itemize}
